# Supplementary material for: Critique-GRPO: Advancing LLM Reasoning with Natural Language and Numerical Feedback
Source: arXiv:2506.03106 source file (2026-06-06)
Supplement: Supplementary file 1 [file appendix_method.tex]

\begin{figure}[th]
\centering
\includegraphics[width=1\linewidth]{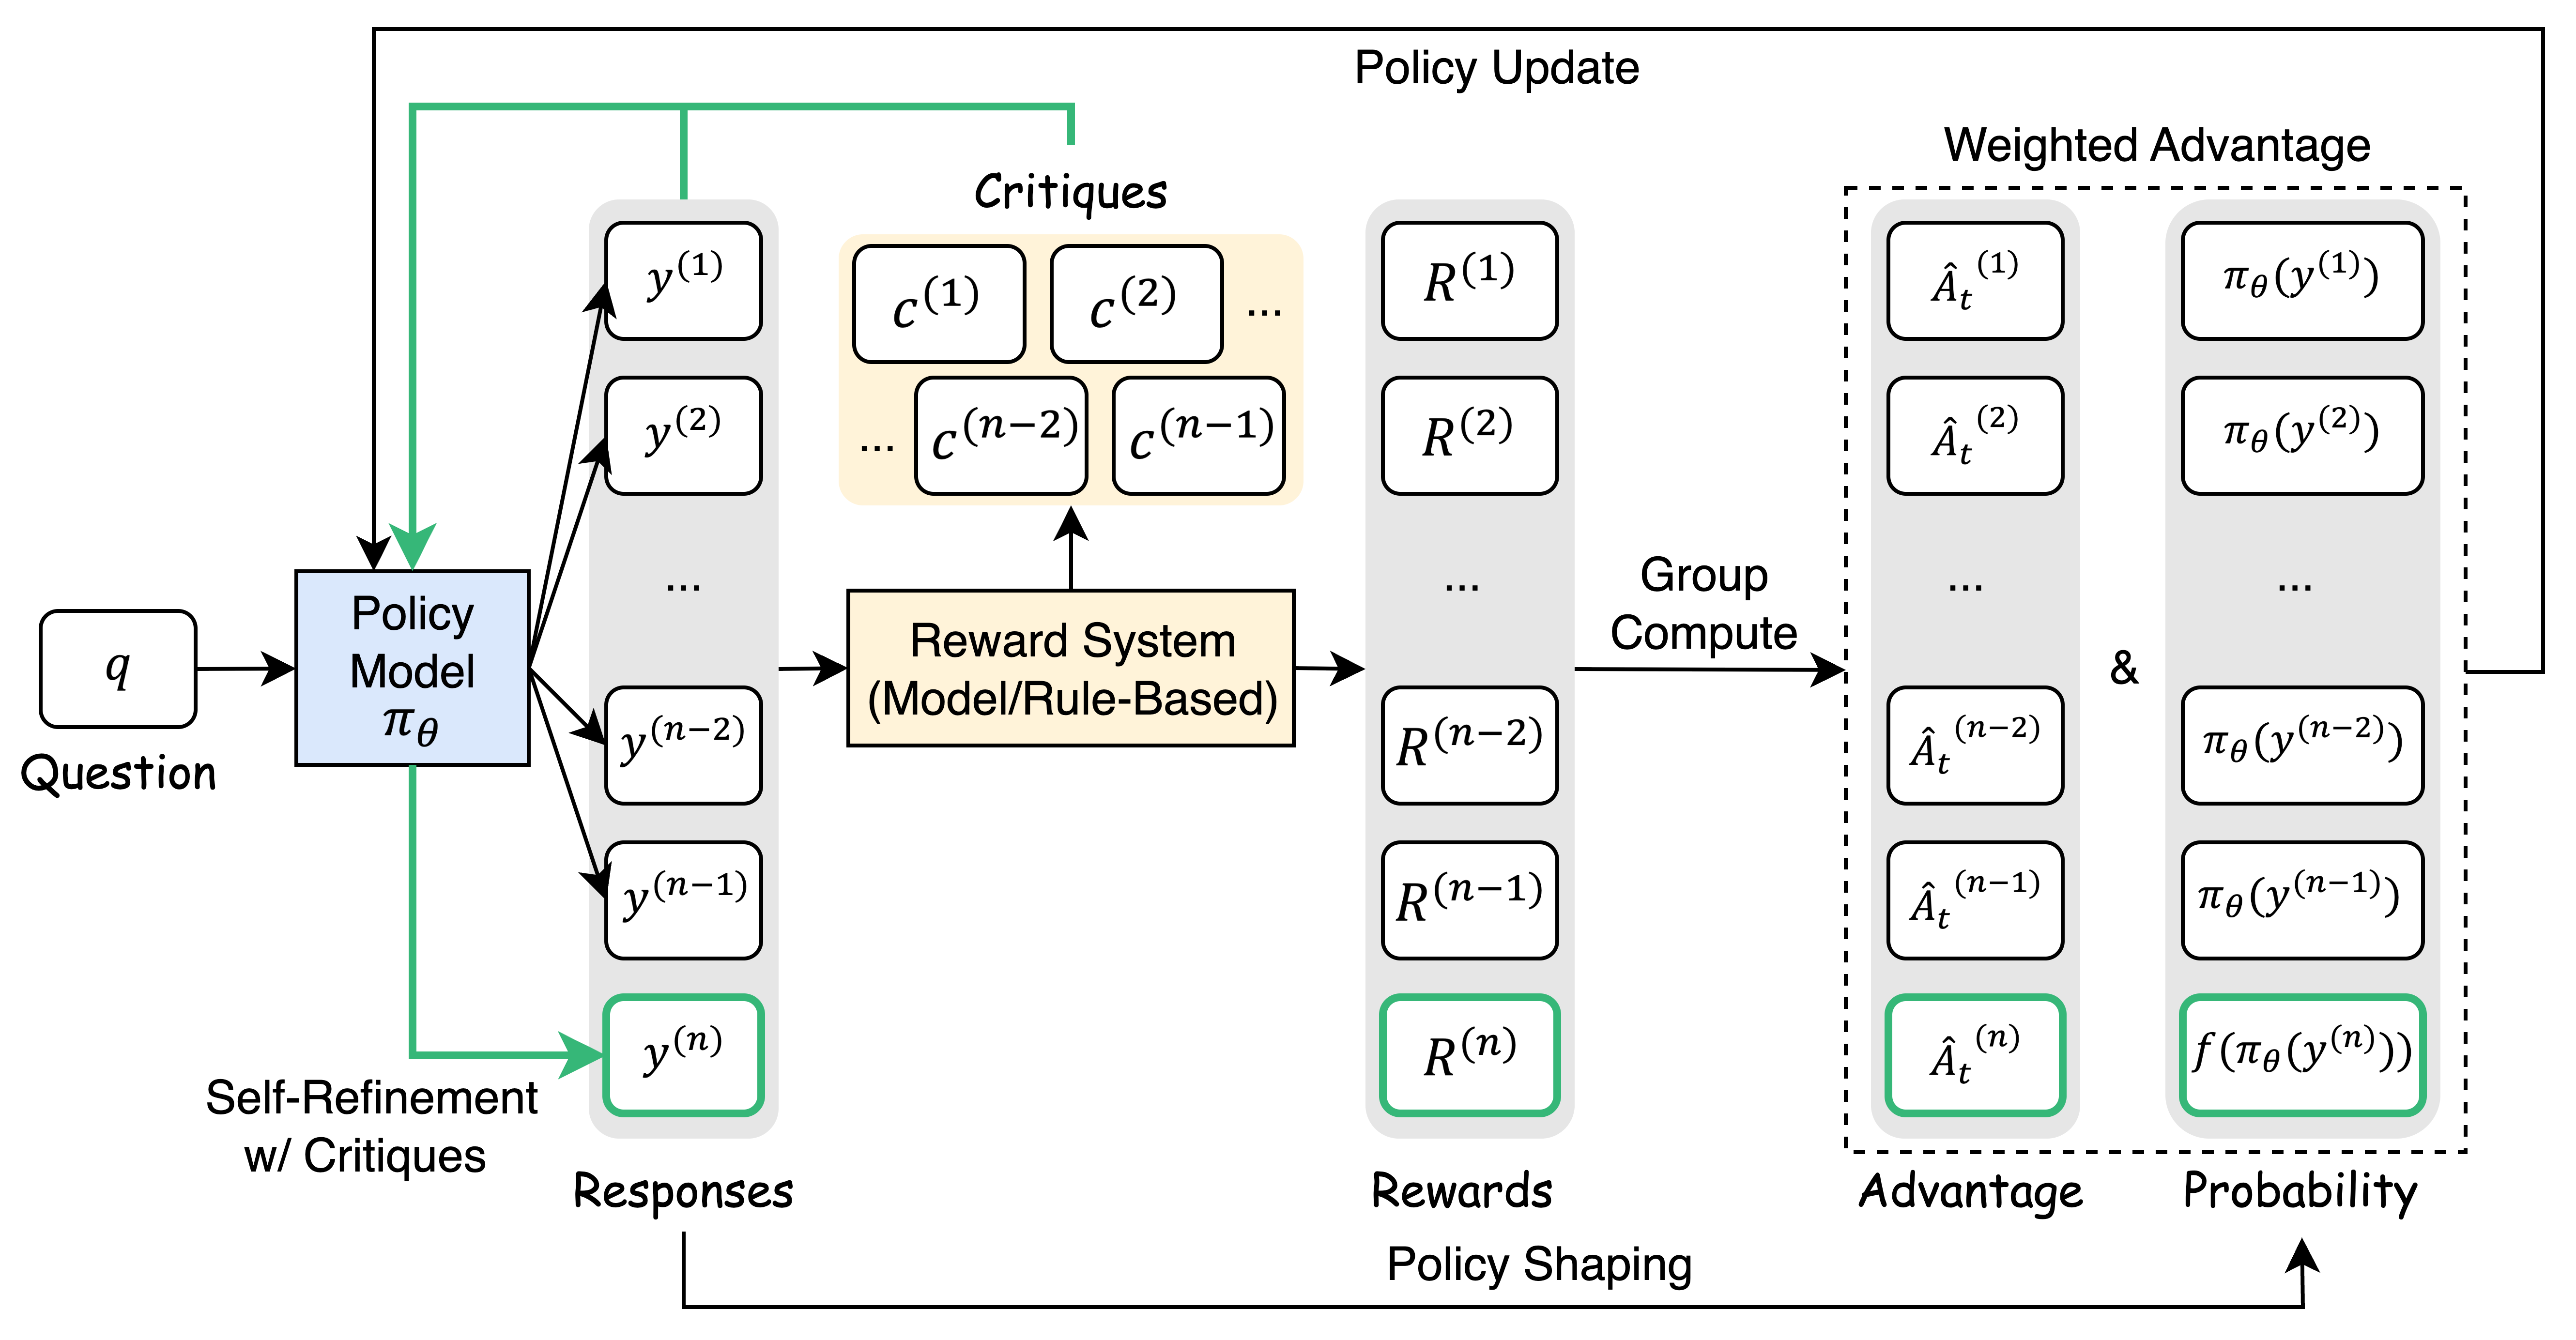} 
\caption{Overview of \critiquegrpo{}. Given a question, \critiquegrpo{} samples initial responses and then refines these responses using critiques generated by a reward system (either model-based or rule-based). These refinements are combined with the initial responses to optimize the policy within an online reinforcement learning framework. A weighted advantage function, combined with policy shaping, emphasizes correct refinements while strongly penalizing incorrect ones.}
\label{fig:critique_grpo}
\end{figure}

% \caption{\critiquegrpo{}: An Overview. Given a question, \critiquegrpo{} samples initial responses and then refines these responses using critiques generated by a reasoning-based reward model. These refinements are combined with the initial responses to optimize the policy within an online reinforcement learning framework. A weighted advantage function, combined with policy shaping, emphasizes correct refinements while strongly penalizing incorrect ones.}
% \label{fig:critique_grpo}

% \begin{figure}[th]
% \centering
% \includegraphics[width=1\linewidth]{floats/raw_figures/critique_grpo.png} 
% \caption{Illustration of \critiquegrpo{}. \critiquegrpo{} leverages critiques from a reasoning-based reward model to refine responses, which are combined with initial solutions within an on-policy optimization reinforcement learning framework. A weighted advantage function with policy shaping is used to emphasize correct refinements while heavily penalizing incorrect ones.}
% \label{fig:critique_grpo}
% \end{figure}

Motivated by the potential of leveraging critiques, particularly CoT critiques, for effective model refinement (Section~\ref{sec:preliminary}), we introduce \critiquegrpo{}, an online optimization algorithm that learns from both natural language and numerical feedback. As illustrated in Figure~\ref{fig:critique_grpo}, \critiquegrpo{} facilitates effective online learning and exploration by enabling the model to learn from both its generated responses and its effective refinements by incorporating natural language feedback (specifically, critiques). Before delving into the details of \critiquegrpo{} (Section~\ref{sec:grpo_to_critique_grpo}), we briefly review Group Relative Policy Optimization (GRPO)~\citep{DBLP:journals/corr/abs-2402-03300} (Section~\ref{sec:online_w_critique_grpo}).

\subsection{From GRPO to \critiquegrpo{}}
\label{sec:grpo_to_critique_grpo}

GRPO is an online RL algorithm widely used during the fine-tuning stage of LLMs. It builds on Proximal Policy Optimization (PPO)~\citep{schulman2017proximalpolicyoptimizationalgorithms}, but eliminates the need for value function approximation by estimating advantages based on the relative performance of groups of actions. In the context of LLM policy optimization, let the model policy be parameterized by $\theta$. For each question $q$ in a given set $Q$, a group of responses $\{y^{(i)}\}_{i=1}^n$ is sampled from the old policy $\pi_{\text{old}}$. A reward model then scores these responses, yielding rewards $\{R^{(i)}\}_{i=1}^n$. The GRPO training objective is formulated as:

\begin{equation}
\begin{aligned}
\mathcal{J}_{\text{GRPO}}(\theta) &= 
\mathbb{E}_{q \sim Q, \{y^{(i)}\}_{i=1}^n \sim \pi_{\text{old}}(\cdot|q)} \\
&
\frac{1}{n} \sum_{i=1}^n \textcolor{gray}{\frac{1}{|y^{(i)}|}} \sum_{t=1}^{|y^{(i)}|} 
\left\{
\min \left[
r_{t}^{(i)}(\theta) \hat{A}_{t}^{(i)}, 
\text{clip}(r_{t}^{(i)}(\theta), 1 - \epsilon, 1 + \epsilon) \hat{A}_{t}^{(i)}
\right]  
- \beta D_{\text{KL}} [\pi_\theta || \pi_{\text{ref}}]
\right\},
\end{aligned}
\end{equation}

where $r_{t}^{(i)}(\theta)$ is the probability ratio, comparing the current policy $\pi_{\theta}$ to the old policy $\pi_{\text{old}}$ from which the responses were sampled:

\begin{equation}
r_{t}^{(i)}(\theta) = \frac{\pi_\theta(y_{t}^{(i)} | q, y_{<t}^{(i)})}{\pi_{\text{old}}(y_{t}^{(i)} | q, y_{<t}^{(i)})}, \quad \text{where } r_{t}^{(i)}(\theta_{\text{old}}) = 1, 
\end{equation}

Here, $\epsilon$ and $\beta$ are hyperparameters. The term $\epsilon$ controls the range of the clipped probability ratio, enforcing a pessimistic lower bound on policy performance to prevent excessively large policy updates. Meanwhile, $\beta$ regulates the KL divergence penalty, constraining the trained policy from deviating significantly from the reference policy.

The advantage $\hat{A}_{t}^{(i)}$ for all tokens in a response is calculated by normalizing the rewards $\{R^{(i)}\}_{i=1}^n$ using the group mean and standard deviation:

\begin{equation}
\hat{A}_{t}^{(i)} = \frac{R^{(i)} - \text{mean}(\{R^{(1)}, \ldots, R^{(n)}\})}{\textcolor{gray}{\text{std}(\{R^{(1)}, \ldots, R^{(n)}\})}}.
\end{equation}

Recent work~\citep{liu2025understandingr1zeroliketrainingcritical} suggests that the token-level normalization and the standard deviation term in the advantage calculation (highlighted in \textcolor{gray}{gray}) may introduce biased optimization. Following their implementation, we remove these terms to obtain an unbiased optimization objective.

\subsection{Online Learning with \critiquegrpo{}}
\label{sec:online_w_critique_grpo}

We introduce \critiquegrpo{}, an online policy optimization framework that enables a model to learn simultaneously from its generated responses and their refinements by incorporating critiques generated by a reasoning-based reward model. This approach helps the model discover new solutions and mitigate repeated failures on specific questions, as discussed in Section~\ref{sec:preliminary}.

Specifically, \critiquegrpo{} operates in three main steps (Figure~\ref{fig:critique_grpo}):

\noindent \textbf{Step 1: Initial Response Sampling.}  
Given an LLM and a set of questions $Q = \{q\}$, we sample $n$ initial responses for each question from the old policy $\pi_{\text{old}}$:  
$\{y^{(i)}\}_{i=1}^{n} \sim \pi_{\text{old}}(\cdot \mid q)$. These responses are evaluated using a reward system to generate both critiques $\{c^{(i)}\}_{i=1}^{n}$ and scalar rewards $\{R^{(i)}\}_{i=1}^{n}$, formulated as: 
\[
c^{(i)}, R^{(i)} \leftarrow \text{Reward}(q, y^{(i)}), \forall i.
\]
We consider two types of reward systems: \textit{model-based} and \textit{rule-based}. $(\RN{1})$ For the model-based reward system, we use a reasoning-based reward model $\pi_{RM}$ to generate CoT critiques: $c_{\text{CoT}}^{(i)} \sim \pi_{RM}(\cdot \mid I_c, q, y^{(i)}),$ where $I_c$ is the critique instruction. These critiques, based on question-response pairs, are described in Appendix~\ref{app:preliminary}. Binary correctness labels from the critiques are converted into scalar reward scores: $R^{(i)} \leftarrow c_{\text{CoT}}^{(i)}$. $(\RN{2})$ For the rule-based reward system, we compare the generated responses against ground-truth answers using a string-matching function to compute scalar rewards: $R^{(i)} = \text{is\_equivalent}(y^{(i)}, y_{\text{GT}}).$\footnote{To ensure consistency, we align the results of model- and rule-based evaluations, isolating the effects of incorporating natural language feedback.} From these evaluations, two heuristic-based critiques, \ie $c_{\text{I}}^{(i)}$ (indicative critique) and $c_{\text{GT}}^{(i)}$ (critique with ground truth) are derived: $c_{\text{I}}^{(i)}, c_{\text{GT}}^{(i)} \leftarrow  R^{(i)}$, as detailed in Appendix~\ref{app:preliminary}.

% $(\RN{1})$ \textbf{Initial Response Sampling:}  
% Given an LLM and a set of questions $Q = \{q\}$, we sample $k$ initial responses for each question from the old policy $\pi_{\text{old}}$: $\{y^{(i)}\}_{i=1}^{n} \sim \pi_{\text{old}}(\cdot|q)$. These responses are scored using a reasoning-based reward model $\pi_\phi$, which generates CoT critiques: $\{c_{\text{CoT}}^{(i)}\}_{i=1}^{n} \sim \pi_\phi(\cdot \mid I_c, q, y^{(i)}),$ based on question-response pair and the critique instruciton $I_{c}$, as illustrated in Section~\ref{sec:preliminary}. The binary correctness labels in these critiques are translated into scalar reward scores $\{R^{(i)}\}_{i=1}^{n}$.

\noindent \textbf{Step 2: Critique-Guided Self-Refinement.}  
Next, we prompt the LLM to generate refined responses conditioned on the question-response-critique triplet $(q, y^{(i)}, c^{(i)})$ and a refinement instruction $I_{\text{refine}}$ (detailed in Appendix~\ref{app:prompts}): $y_{\text{refined}}^{(i)} \sim \pi_{\text{old}}(\cdot \mid I_{\text{refine}}, q, y^{(i)}, c^{(i)}),$ where $c^{(i)} \in \{c_{\text{CoT}}^{(i)}, c_{\text{GT}}^{(i)}, c_{\text{I}}^{(i)}\}$. The reward model scores these self-generated refinements, producing $\{R_{\text{refine}}^{(i)}\}_{i=1}^{n}$ (alternatively, the rule-based evaluation function discussed in Appendix~\ref{app:preliminary} could be used). To mitigate potential distributional shifts induced by the refinements, we randomly sample a subset of $k$ refinements, denoted by $\{y_{\text{refined}}^{(i')}\}_{i'=1}^{k}$, from the full refinement set $\{y_{\text{refined}}^{(i)}\}_{i=1}^{n}$. This sampling prioritizes correct refinements; if no correct refinements are generated, incorrect refinements are sampled randomly. We then combine the sampled subset of refinements with the initial responses to form a mixed group of responses.\footnote{Currently, only one refined response is retained. Future work may explore the optimal data ratio.}

\noindent \textbf{Step 3: Online Policy Optimization.} 
Finally, the model is fine-tuned on a mixed set of initial and refined responses using scalar rewards. The training objective, adapted from GRPO, is given by:
\begin{equation}
\begin{aligned}
\mathcal{J}_{\text{Critique-GRPO}}(\theta) = 
&\ \mathbb{E}_{q \sim Q, \{y^{(i)}\}_{i=1}^{n} \sim \pi_{\text{old}}(\cdot \mid q), \{y_{\text{refined}}^{(i')}\}_{i'=1}^{k} \sim \pi_{\text{old}}(\cdot \mid q)} \bigg[ \\
&\quad \underbrace{\frac{1}{n} \sum_{i=1}^n \sum_{t=1}^{|y^{(i)}|} \min \left[
r_{t}^{(i)}(\theta) \hat{A}_{t}^{(i)}, 
\text{clip}(r_{t}^{(i)}(\theta), 1 - \epsilon, 1 + \epsilon) \hat{A}_{t}^{(i)}
\right]}_{\text{Objective for Initial Responses}} \\
&\quad + \underbrace{\frac{1}{k} \sum_{i'=1}^k \sum_{t=1}^{|y_{\text{refined}}^{(i')}|} \min \left[
r_{\text{refined}, t}^{(i')}(\theta) A_{t}^{(i')}, 
\text{clip}(r_{\text{refined}, t}^{(i')}(\theta), 1 - \epsilon, 1 + \epsilon) A_{t}^{(i')}
\right]}_{\text{Objective for Refined Responses}} 
\bigg].
\label{critique-grpo-loss}
\end{aligned}
\end{equation}

where the advantages $A_{t}^{(i)}$, $A_{t}^{(i')}$ for all tokens in a response are defined as:
 
\begin{equation}
\begin{aligned}
    A_{t}^{(i)} &= R^{(i)} - \text{mean} \big( \{R^{(j)}\}_{j=1}^{n} \cup \{R_{\text{refined}}^{(j')}\}_{j'=1}^{k} \big), \\
    A_{t}^{(i')} &= R^{(i')} - \text{mean} \big( \{R^{(j)}\}_{j=1}^{n} \cup \{R_{\text{refined}}^{(j')}\}_{j'=1}^{k} \big),
\end{aligned}
\end{equation}

$r_{t}^{(i)}(\theta)$ and $f(r_{\text{refined}, t}^{(i')}(\theta))$ represent the token-level probability ratios:

\begin{equation}
r_{t}^{(i)}(\theta) = \frac{\pi_\theta(y_{t}^{(i)} | q, y_{<t}^{(i)})}{\pi_{\text{old}}(y_{t}^{(i)} | q, y_{<t}^{(i)})}, \quad 
f(r_{\text{refined}, t}^{(i')}(\theta)) = \frac{\pi_\theta(y_{\text{refined}, t}^{(i')} | q, y_{\text{refined}, <t}^{(i')})}{\pi_\theta(y_{\text{refined}, t}^{(i')} | q, y_{\text{refined}, <t}^{(i')}) + \gamma}.
\end{equation}

We adopt a shaping function $f(x) = x/(x+\gamma)$\citep{yan2025learningreasonoffpolicyguidance} ($0<\gamma<1$), depicted in Figure\ref{fig:shaping_function} and the lower right corner of Figure~\ref{fig:critique_grpo}, to reweight gradients and emphasize low-probability tokens in refined responses. As illustrated in Figure~\ref{fig:shaping_function}, this function is bounded between $(0,1)$, where $x$ represents the token probability of the policy. When $\gamma$ is small (\ie 0.1), the function significantly amplifies low probabilities, with this amplification decreasing as $x$ increases. Larger $\gamma$ values (0.9) produce less pronounced scaling effects. The black dashed diagonal line indicates no shaping (\ie $f(x) = x$). 

\input{floats/figures/figure_shaping_function}

We set $\gamma=0.1$ to optimize learning from unfamiliar yet correct refinements while strongly penalizing unfamiliar incorrect ones. Additionally, we remove the KL-divergence penalty term from the original GRPO formulation to reduce constraints on policy updates, enabling more substantial model adjustments and effective learning from refinements. Future work may explore the use of the clip-high strategy~\citep{yu2025dapoopensourcellmreinforcement} to reduce update constraints. We summarize \critiquegrpo{} in Algorithm~\ref{alg:critique_grpo} (Appendix~\ref{app:algorithm_critique_grpo}).

We also experiment with the ratio of initial responses to refinements per prompt, ranging from 1:1 to 7:1. Our results indicate that a 7:1 ratio achieves both stable training and optimal performance. Lower ratios lead to performance degradation due to sudden increases in entropy loss, caused by distribution shifts introduced by the refinements, during later training stages.
