# Supplementary material for: Critique-GRPO: Advancing LLM Reasoning with Natural Language and Numerical Feedback
Source: arXiv:2506.03106 source file (2026-06-06)
Supplement: Supplementary file 2 [file appendix_theoretical_analysis.tex]

We analyze the learning dynamics of \textsc{Critique-GRPO} by modeling the LLM fine-tuning process as a Contextual Bandit problem~\citep{may2012optimistic} with Version Spaces~\citep{mitchell1979version}. This abstraction captures the core advantage of our approach: while scalar rewards ($r$) provide information about \textit{utility}, language feedback (critiques, $o$) provides information about \textit{structure}, allowing the learner to eliminate suboptimal hypotheses that are indistinguishable via scalar rewards alone.

\subsection{Problem Formulation}

Let $\mathcal{A}$ be the action space (generated responses) and $\mathcal{H}$ be a hypothesis class of reward functions. The true environment is governed by a hidden parameter $\theta^* \in \mathcal{H}$. At each step $t$:
\begin{enumerate}
    \item The agent selects an action $a_t \in \mathcal{A}$.
    \item The environment provides a noisy scalar reward $r_t = r(a_t; \theta^*) + \eta_t$, where $\eta_t$ is $\sigma^2$-sub-Gaussian noise.
    \item \textbf{(Hybrid Only)} The environment provides language feedback (critique) $o_t$, sampled from a distribution $P(\cdot \mid a_t; \theta^*)$.
\end{enumerate}

We compare two learners: the \textbf{Numerical Learner} ($\pi_{\text{num}}$), which updates its belief based solely on history $H_t^{\text{num}} = \{(a_\tau, r_\tau)\}_{\tau=1}^{t-1}$, and the \textbf{Hybrid Learner} ($\pi_{\text{hybrid}}$), which utilizes $H_t^{\text{hybrid}} = \{(a_\tau, r_\tau, o_\tau)\}_{\tau=1}^{t-1}$.

\subsection{Confidence Sets and Intersection}

We utilize the framework of Version Spaces. A confidence set represents the subset of hypotheses in $\mathcal{H}$ that remain consistent with the observed history.

\begin{definition}[Numerical Confidence Set]
The set of hypotheses consistent with the scalar rewards up to time $t$ is defined by the least-squares error bound:
\begin{equation}
    C_t^{\text{num}} = \left\{ \theta \in \mathcal{H} : \sum_{\tau=1}^{t-1} \left( r(a_\tau; \theta) - r_\tau \right)^2 \le \beta_t \right\}
\end{equation}
where $\beta_t$ is a confidence radius chosen to ensure $\theta^* \in C_t^{\text{num}}$ with high probability.
\end{definition}

\begin{definition}[Language Consistency Set]
The set of hypotheses consistent with the language feedback is defined by the log-likelihood of the observed critiques:
\begin{equation}
    C_t^{\text{lang}} = \left\{ \theta \in \mathcal{H} : \sum_{\tau=1}^{t-1} -\log P(o_\tau \mid a_\tau; \theta) \le \gamma_t \right\}
\end{equation}
\end{definition}

\begin{definition}[Hybrid Confidence Set]
The Hybrid Learner operates on the \textbf{intersection} of these constraints:
\begin{equation}
    C_t^{\text{hybrid}} = C_t^{\text{num}} \cap C_t^{\text{lang}}
\end{equation}
\end{definition}

\subsection{Regret Analysis}

We analyze the regret $R_T = \sum_{t=1}^T (\max_{a} r(a; \theta^*) - r(a_t; \theta^*))$. We assume the learner follows an Optimism in the Face of Uncertainty (OFU) strategy~\citep{neu2020unifying}, selecting actions that maximize the potential reward within the confidence set.

\begin{theorem}[Weak Dominance]
\label{thm:weak_dominance}
For any time horizon $T$, the regret of the Hybrid Learner is bounded by the regret of the Numerical Learner:
\begin{equation}
    R_T(\pi_{\text{hybrid}}) \le R_T(\pi_{\text{num}})
\end{equation}
\end{theorem}

\begin{proof}
By definition, $C_t^{\text{hybrid}} = C_t^{\text{num}} \cap C_t^{\text{lang}}$, which implies $C_t^{\text{hybrid}} \subseteq C_t^{\text{num}}$.
The uncertainty width of a confidence set $C$ for action $a$ is $w(C, a) = \sup_{\theta_1, \theta_2 \in C} |r(a; \theta_1) - r(a; \theta_2)|$.
Since the supremum over a subset is less than or equal to the supremum over the superset, $w(C_t^{\text{hybrid}}, a_t) \le w(C_t^{\text{num}}, a_t)$.
Standard bandit analysis bounds regret by the sum of these widths. Thus, the Hybrid regret is strictly upper-bounded by the Numerical regret.
\end{proof}

\begin{theorem}[Strict Improvement via Orthogonality]
\label{thm:strict_improvement}
Assume the language feedback is \textbf{$\epsilon$-informative}~\citep{xu2025provablylearninglanguagefeedback}: there exists a confusing hypothesis $\theta \neq \theta^*$ such that $|r(a; \theta) - r(a; \theta^*)| \le \epsilon$ (rewards are indistinguishable) but $D_{\text{KL}}(P(\cdot|a;\theta^*) || P(\cdot|a;\theta)) \ge \Delta > 0$ (feedback is distinct).
Then, there exist problem instances where:
\begin{equation}
    R_T(\pi_{\text{hybrid}}) = O(\log T) \quad \text{while} \quad R_T(\pi_{\text{num}}) = \Omega(T)
\end{equation}
\end{theorem}

\begin{proof}
\textbf{Numerical Failure:} If $|r(a; \theta) - r(a; \theta^*)|$ is negligible, the scalar reward signal is insufficient to distinguish the suboptimal hypothesis $\theta$ from the optimal $\theta^*$. The Numerical Learner keeps $\theta$ in $C_t^{\text{num}}$, potentially choosing suboptimal actions associated with $\theta$ indefinitely (linear regret).

\textbf{Hybrid Success:} The language feedback provides a constant information gain $\Delta$ per step. The likelihood constraint in $C_t^{\text{lang}}$ forces the probability mass of $\theta$ to decay exponentially. Consequently, $\theta$ is rapidly eliminated from the intersection $C_t^{\text{hybrid}}$, reducing the problem to the standard logarithmic regret regime.
\end{proof}

\subsection{Sample Complexity: The "Needle in a Haystack" Separation}

To illustrate the magnitude of this improvement in the context of reasoning tasks (e.g., code generation), we present a simplified complexity analysis.

\begin{proposition}
Let $\mathcal{H} = \{0, 1\}^d$ be the hypothesis space (e.g., binary decisions in a reasoning trace). Let the reward be sparse: $r(a) = \mathbb{1}\{a = \theta^*\}$. Let the critique $o_t$ indicate the index of the first incorrect bit. To identify $\theta^*$ with probability $1-\delta$:
\begin{itemize}
    \item \textbf{Numerical Learner:} Requires $\Omega(2^d)$ samples (Exhaustive Search).
    \item \textbf{Hybrid Learner:} Requires $O(d)$ samples (Binary Search).
\end{itemize}
\end{proposition}

\begin{proof}
\textbf{Numerical:} Observing $r(a)=0$ only eliminates the single hypothesis $a$. The version space shrinks linearly: $|C_t| = 2^d - t$.
\textbf{Hybrid:} A critique "Bit $i$ is wrong" eliminates all hypotheses where the $i$-th bit matches $a_i$. This acts as a hyperplane cut, halving the search space (or fixing one dimension) at each step. The version space shrinks exponentially.
\end{proof}

\subsection{Connection to \textsc{Critique-GRPO}}

This theoretical framework maps directly to our algorithm:
\begin{enumerate}
    \item \textbf{Intersection ($C^{\text{num}} \cap C^{\text{lang}}$):} \textsc{Critique-GRPO} uses the critique to generate a refined response. The model update is driven not just by the reward of the original response, but by the \textit{contrast} between the original and the critique-guided response. This effectively constrains the policy update to the intersection of "high reward" and "critique-consistent" regions.
    \item \textbf{Orthogonal Information:} In reasoning tasks, a "correct answer" (reward) often fails to reveal \textit{why} a step was valid. The critique provides the causal reasoning (the $\epsilon$-informative signal), allowing the model to generalize the logic rather than just memorizing the answer.
\end{enumerate}
