# Supplementary material for: Critique-GRPO: Advancing LLM Reasoning with Natural Language and Numerical Feedback
Source: arXiv:2506.03106 source file (2026-06-06)
Supplement: Supplementary file 3 [file new_appendix_theoretical_analysis.tex]

We analyze the learning dynamics of \textsc{Critique-GRPO} by modeling the LLM fine-tuning process as a Contextual Bandit problem~\citep{may2012optimistic} augmented with Version Spaces~\citep{mitchell1979version}. This abstraction captures the core advantage of our approach: while scalar rewards ($r$) provide information about \textit{utility}, language feedback (critiques, $o$) provides information about \textit{structure}, allowing the learner to eliminate suboptimal hypotheses that are indistinguishable via scalar rewards alone.

\subsection{Problem Formulation}

Let $\mathcal{A}$ be the action space (generated responses) and $\mathcal{H}$ be a hypothesis class of reward functions. The true environment is governed by a hidden parameter $\theta^* \in \mathcal{H}$. At each step $t$:
\begin{enumerate}
    \item The agent selects an action $a_t \in \mathcal{A}$.
    \item The environment provides a noisy scalar reward $r_t = r(a_t; \theta^*) + \eta_t$, where $\eta_t$ is sub-Gaussian noise with parameter $\sigma^2$.
    \item \textbf{(Hybrid Only)} The environment provides language feedback (critique) $o_t$, sampled from a distribution $P(\cdot \mid a_t; \theta^*)$.
\end{enumerate}

We compare two learners: the \textbf{Numerical Learner} ($\pi_{\text{num}}$), which updates its belief based solely on history $H_t^{\text{num}} = \{(a_\tau, r_\tau)\}_{\tau=1}^{t-1}$, and the \textbf{Hybrid Learner} ($\pi_{\text{hybrid}}$), which utilizes $H_t^{\text{hybrid}} = \{(a_\tau, r_\tau, o_\tau)\}_{\tau=1}^{t-1}$.

\subsection{Confidence Sets and Version Space Intersection}

We utilize the framework of Version Spaces~\citep{mitchell1979version} to model the set of hypotheses consistent with observations.

\begin{definition}[Confidence Sets]
\label{def:confidence_sets}
At time $t$, we define the confidence sets constrained by utility and structure respectively:
\begin{align}
    C_t^{\text{num}} &= \left\{ \theta \in \mathcal{H} : \sum_{\tau=1}^{t-1} \left( r(a_\tau; \theta) - r_\tau \right)^2 \le \beta_t \right\} \quad \text{(Utility Constraint)} \\
    C_t^{\text{lang}} &= \left\{ \theta \in \mathcal{H} : \sum_{\tau=1}^{t-1} -\log P(o_\tau \mid a_\tau; \theta) \le \gamma_t \right\} \quad \text{(Structural Constraint)}
\end{align}
where $\beta_t = O(\sigma^2 \log(|\mathcal{H}|t/\delta))$ and $\gamma_t = O(\log(|\mathcal{H}|t/\delta))$ are concentration parameters ensuring that $\theta^* \in C_t^{\text{num}}$ and $\theta^* \in C_t^{\text{lang}}$ with probability at least $1-\delta$.

The Hybrid Learner operates on the \textbf{intersection}:
\begin{equation}
C_t^{\text{hybrid}} = C_t^{\text{num}} \cap C_t^{\text{lang}}
\end{equation}
\end{definition}

\begin{lemma}[Volume Reduction]
\label{lem:volume_reduction}
The volume of the hybrid confidence set is bounded by:
\begin{equation}
\text{Vol}(C_t^{\text{hybrid}}) = \text{Vol}(C_t^{\text{num}} \cap C_t^{\text{lang}}) \le \min(\text{Vol}(C_t^{\text{num}}), \text{Vol}(C_t^{\text{lang}}))
\end{equation}
Moreover, when the language feedback is informative (i.e., $C_t^{\text{lang}}$ imposes non-redundant constraints), we have:
\begin{equation}
\text{Vol}(C_t^{\text{hybrid}}) \le \text{Vol}(C_t^{\text{num}}) \cdot \exp\left(-\sum_{\tau=1}^{t-1} I(o_\tau; \theta^* \mid a_\tau)\right)
\end{equation}
where $I(o_\tau; \theta^* \mid a_\tau) \ge 0$ is the information gain from language feedback.
\end{lemma}

\begin{proof}
The first inequality follows directly from set theory. For the second, consider the posterior distribution $P(\theta \mid H_t^{\text{hybrid}})$. By Bayes' rule:
\begin{align}
P(\theta \mid H_t^{\text{hybrid}}) &\propto P(\theta) \prod_{\tau=1}^{t-1} P(r_\tau \mid a_\tau, \theta) \cdot P(o_\tau \mid a_\tau, \theta)
\end{align}
The entropy reduction from language feedback is:
\begin{align}
H(\theta \mid H_t^{\text{num}}) - H(\theta \mid H_t^{\text{hybrid}}) = \sum_{\tau=1}^{t-1} I(o_\tau; \theta \mid a_\tau, r_\tau)
\end{align}
Since volume scales exponentially with entropy in high-dimensional spaces, we obtain the stated bound.
\end{proof}

\subsection{Regret Analysis and Weak Dominance}

We analyze the cumulative regret $R_T = \sum_{t=1}^T (\max_{a} r(a; \theta^*) - r(a_t; \theta^*))$. We assume both learners follow an Optimism in the Face of Uncertainty (OFU) strategy, selecting actions that maximize the optimistic reward estimate within their respective confidence sets.

\begin{theorem}[Weak Dominance]
\label{thm:weak_dominance}
For any time horizon $T$, the regret of the Hybrid Learner is bounded by the regret of the Numerical Learner:
\begin{equation}
R_T(\pi_{\text{hybrid}}) \le R_T(\pi_{\text{num}})
\end{equation}
\end{theorem}

\begin{proof}
By Definition~\ref{def:confidence_sets}, we have $C_t^{\text{hybrid}} \subseteq C_t^{\text{num}}$ for all $t$. 

Define the uncertainty width of a confidence set $C$ for action $a$ as:
\begin{equation}
w(C, a) = \sup_{\theta_1, \theta_2 \in C} |r(a; \theta_1) - r(a; \theta_2)|
\end{equation}

Under the OFU principle, the per-step regret is bounded by:
\begin{equation}
r(a_t^*; \theta^*) - r(a_t; \theta^*) \le w(C_t, a_t)
\end{equation}
where $a_t^* = \arg\max_a r(a; \theta^*)$ is the optimal action.

Since $C_t^{\text{hybrid}} \subseteq C_t^{\text{num}}$, we have for any action $a$:
\begin{equation}
w(C_t^{\text{hybrid}}, a) = \sup_{\theta_1, \theta_2 \in C_t^{\text{hybrid}}} |r(a; \theta_1) - r(a; \theta_2)| \le \sup_{\theta_1, \theta_2 \in C_t^{\text{num}}} |r(a; \theta_1) - r(a; \theta_2)| = w(C_t^{\text{num}}, a)
\end{equation}

Therefore, at each step $t$:
\begin{equation}
\text{regret}_t(\pi_{\text{hybrid}}) \le w(C_t^{\text{hybrid}}, a_t) \le w(C_t^{\text{num}}, a_t) \le \text{regret}_t(\pi_{\text{num}})
\end{equation}

Summing over all time steps yields the result.
\end{proof}

\subsection{Discriminative Power in Group-Relative Learning}

In GRPO, the policy update is driven by group-relative advantages. We now formalize how language feedback amplifies the discriminative power within groups.

\begin{definition}[$\epsilon$-Informative Critique]
\label{def:informative_critique}
A critique $o$ for action $a$ is called $\epsilon$-informative if there exists a confusing hypothesis $\theta \neq \theta^*$ such that:
\begin{enumerate}
    \item \textbf{Reward Indistinguishability:} $|r(a; \theta) - r(a; \theta^*)| \le \epsilon$
    \item \textbf{Structural Distinguishability:} $D_{\text{KL}}(P(\cdot \mid a; \theta^*) \| P(\cdot \mid a; \theta)) \ge \Delta > 0$
\end{enumerate}
\end{definition}

\begin{lemma}[Discriminative Gap Expansion]
\label{lem:gap_expansion}
Consider a group $G = \{a_1, \ldots, a_{|G|}\}$ with scalar rewards $r_1, \ldots, r_{|G|}$ and corresponding critiques $o_1, \ldots, o_{|G|}$. Define the structural distance induced by critique-guided refinements as:
\begin{equation}
d_{\text{struct}}(a_i, a_j) = \mathbb{E}_{\theta \sim P(\cdot \mid H_t^{\text{hybrid}})} [|r(y_{\text{ref}}^i; \theta) - r(y_{\text{ref}}^j; \theta)|]
\end{equation}
where $y_{\text{ref}}^i$ is the refinement obtained by applying critique $o_i$ to response $a_i$.

If the critiques are $\epsilon$-informative, then the effective discriminative gap in the hybrid space satisfies:
\begin{equation}
\Delta_{\text{hybrid}}(a_i, a_j) \ge \Delta r_{ij} + \lambda \cdot d_{\text{struct}}(a_i, a_j)
\end{equation}
where $\Delta r_{ij} = |r(a_i) - r(a_j)|$ and $\lambda = \Theta(\Delta / \epsilon)$.
\end{lemma}

\begin{proof}
Consider two actions $a_i, a_j$ with similar scalar rewards: $\Delta r_{ij} \le \epsilon$. Without language feedback, the numerical learner cannot distinguish them, leading to $\nabla_\theta \log \pi_\theta(a_i) \approx \nabla_\theta \log \pi_\theta(a_j)$ in the gradient update.

With critiques, the refinements $y_{\text{ref}}^i, y_{\text{ref}}^j$ are generated. By Definition~\ref{def:informative_critique}, there exists $\theta \in C_t^{\text{lang}}$ such that:
\begin{equation}
D_{\text{KL}}(P(\cdot \mid a_i; \theta^*) \| P(\cdot \mid a_i; \theta)) \ge \Delta
\end{equation}

This KL divergence implies that the likelihood ratio $\frac{P(o_i \mid a_i; \theta^*)}{P(o_i \mid a_i; \theta)}$ deviates significantly from 1. By Pinsker's inequality:
\begin{equation}
\| P(\cdot \mid a_i; \theta^*) - P(\cdot \mid a_i; \theta) \|_1 \ge \sqrt{2 \Delta}
\end{equation}

This translates to a structural separation in the space of refinements. Specifically, with probability at least $\sqrt{2\Delta}$, the refinements $y_{\text{ref}}^i, y_{\text{ref}}^j$ will differ in their logical structure, leading to:
\begin{equation}
d_{\text{struct}}(a_i, a_j) \ge c \cdot \sqrt{\Delta}
\end{equation}
for some constant $c > 0$.

In the GRPO gradient update, the advantage of $a_i$ relative to the group mean is:
\begin{equation}
A(a_i) = r(a_i) - \bar{r}_G + \Phi(o_i)
\end{equation}
where $\Phi(o_i)$ encodes the structural information. When critiques are informative, $\Phi(o_i) \neq \Phi(o_j)$ even when $r(a_i) \approx r(a_j)$, yielding:
\begin{equation}
|A(a_i) - A(a_j)| \ge \Delta r_{ij} + \lambda \cdot d_{\text{struct}}(a_i, a_j)
\end{equation}
where $\lambda = \Theta(\Delta / \epsilon)$ captures the relative importance of structural information.
\end{proof}

\subsection{Exponential Separation in Search Complexity}

We now formalize the "Needle in a Haystack" intuition: language feedback transforms exhaustive search into binary search.

\begin{theorem}[Exponential Sample Complexity Separation]
\label{thm:exponential_separation}
Consider a tree-structured reasoning space with $d$ critical decision nodes, where each node has branching factor $b$. The total action space has size $|\mathcal{A}| = b^d$. Assume:
\begin{enumerate}
    \item There exists a unique optimal trajectory $a^*$.
    \item Scalar rewards are binary: $r(a) = 1$ if $a = a^*$, else $r(a) = 0$.
    \item Critiques are $\epsilon$-informative with $\epsilon = o(1/d)$, and identify the first error node along a trajectory.
\end{enumerate}

Then, to identify $a^*$ with probability at least $1-\delta$:
\begin{itemize}
    \item \textbf{Numerical Learner:} Requires $T_{\text{num}} = \Omega(b^d)$ samples in expectation.
    \item \textbf{Hybrid Learner:} Requires $T_{\text{hybrid}} = O(d \cdot \log(1/\delta))$ samples.
\end{itemize}
\end{theorem}

\begin{proof}
\textbf{Lower Bound for Numerical Learner:}

With binary rewards, each failed attempt $a \neq a^*$ provides the information that exactly one trajectory is incorrect. The version space shrinks as:
\begin{equation}
|C_t^{\text{num}}| = |\mathcal{A}| - t = b^d - t
\end{equation}

To reduce the version space to a single hypothesis, we need:
\begin{equation}
T_{\text{num}} \ge |\mathcal{A}| - 1 = b^d - 1 = \Omega(b^d)
\end{equation}

This is an exhaustive search in the worst case.

\textbf{Upper Bound for Hybrid Learner:}

Each critique $o_t$ identifies the first error node $i^*$ in trajectory $a_t$. This acts as a hyperplane cut in the hypothesis space: all trajectories that agree with $a_t$ up to node $i^*$ but differ at node $i^*$ are eliminated.

At node $i^*$, there are $b$ possible choices. The critique eliminates $(b-1)$ branches. The remaining hypotheses consistent with the critique form a subset:
\begin{equation}
|C_t^{\text{lang}}| \le |C_{t-1}^{\text{lang}}| \cdot \left(1 - \frac{b-1}{b}\right) = |C_{t-1}^{\text{lang}}| / b
\end{equation}

At each level $i \in \{1, \ldots, d\}$, the learner needs $O(\log b)$ samples to identify the correct branch with confidence $1 - \delta/d$ (by Hoeffding's inequality). Across all $d$ nodes, the total sample complexity is:
\begin{equation}
T_{\text{hybrid}} = O(d \cdot \log b \cdot \log(d/\delta)) = O(d \cdot \log(1/\delta))
\end{equation}

This binary search strategy achieves exponential improvement: $T_{\text{hybrid}} / T_{\text{num}} = O(d \log b / b^d)$.
\end{proof}

\begin{remark}
The exponential separation is achieved because critiques provide \textbf{structural credit assignment}: they identify \textit{which} part of the reasoning chain failed, not just \textit{that} it failed. This transforms the problem from unstructured exploration over $|\mathcal{A}|$ trajectories to structured exploration over $d$ nodes.
\end{remark}

\subsection{Gradient Consistency in Value-Free Learning}

Unlike Actor-Critic methods that introduce reward modeling error~\citep{azar2023general}, \textsc{Critique-GRPO} directly incorporates structural feedback into the policy gradient without an intermediate value function.

\begin{lemma}[Bias-Free Structural Gradient]
\label{lem:bias_free}
The gradient update in \textsc{Critique-GRPO} can be written as:
\begin{equation}
\nabla_{\theta} J \approx \frac{1}{|G|} \sum_{i=1}^{|G|} \nabla_{\theta} \log \pi_{\theta}(a_i | x) \cdot \left(r(a_i) - \bar{r}_G + \Phi(o_i)\right)
\end{equation}
where $\bar{r}_G = \frac{1}{|G|} \sum_{j=1}^{|G|} r(a_j)$ and $\Phi(o_i)$ encodes the critique-induced refinement signal.

Under the assumption that critiques are unbiased indicators of structural quality (i.e., $\mathbb{E}[\Phi(o_i) \mid a_i, \theta^*] = \mathbb{E}[r(y_{\text{ref}}^i; \theta^*) - r(a_i; \theta^*)]$), this gradient is an unbiased estimator of:
\begin{equation}
\nabla_{\theta} \mathbb{E}_{a \sim \pi_\theta} [r(a; \theta^*) + \mathbb{E}_{o \sim P(\cdot \mid a; \theta^*)}[\Delta r_{\text{ref}}(a, o)]]
\end{equation}
where $\Delta r_{\text{ref}}(a, o) = r(y_{\text{ref}}; \theta^*) - r(a; \theta^*)$ is the improvement from refinement.
\end{lemma}

\begin{proof}
The standard GRPO gradient is:
\begin{equation}
\nabla_{\theta} J_{\text{GRPO}} = \mathbb{E}_{x \sim \mathcal{D}, G \sim \pi_\theta^{|G|}} \left[ \frac{1}{|G|} \sum_{i=1}^{|G|} \nabla_{\theta} \log \pi_{\theta}(a_i | x) \cdot (r(a_i) - \bar{r}_G) \right]
\end{equation}

In \textsc{Critique-GRPO}, we augment the advantage with the critique signal $\Phi(o_i)$. To show this is unbiased, we need:
\begin{equation}
\mathbb{E}_{o_i \sim P(\cdot \mid a_i; \theta^*)} [\Phi(o_i)] = \mathbb{E}_{o_i} [r(y_{\text{ref}}^i; \theta^*) - r(a_i; \theta^*)]
\end{equation}

By construction, the refinement $y_{\text{ref}}^i$ is generated by applying the critique $o_i$ to $a_i$. If the critique provides actionable feedback, then with high probability:
\begin{equation}
r(y_{\text{ref}}^i; \theta^*) \ge r(a_i; \theta^*)
\end{equation}

Taking expectations:
\begin{align}
\mathbb{E}_{a, o} [\nabla_{\theta} \log \pi_{\theta}(a | x) \cdot \Phi(o)] &= \mathbb{E}_{a, o} [\nabla_{\theta} \log \pi_{\theta}(a | x) \cdot (r(y_{\text{ref}}; \theta^*) - r(a; \theta^*))] \\
&= \mathbb{E}_{a} [\nabla_{\theta} \log \pi_{\theta}(a | x) \cdot \mathbb{E}_{o \mid a}[\Delta r_{\text{ref}}(a, o)]]
\end{align}

This is an unbiased estimator of the gradient of the augmented objective, which maximizes both immediate reward and expected improvement from refinement.
\end{proof}

\subsection{Connection to \textsc{Critique-GRPO}}

This theoretical framework directly supports the practical algorithm:

\begin{enumerate}
    \item \textbf{Intersection Principle (Theorem~\ref{thm:weak_dominance}):} The critique-guided refinement mechanism in \textsc{Critique-GRPO} implicitly constructs $C_t^{\text{hybrid}} = C_t^{\text{num}} \cap C_t^{\text{lang}}$. The policy update is driven by the contrast between original responses (constrained by $C_t^{\text{num}}$) and refinements (constrained by $C_t^{\text{lang}}$), ensuring convergence to the intersection region.

    \item \textbf{Exponential Speedup (Theorem~\ref{thm:exponential_separation}):} In complex reasoning tasks (e.g., mathematics, coding), a correct final answer often fails to reveal \textit{why} intermediate steps are valid. Critiques provide structural credit assignment, enabling the model to learn generalizable reasoning patterns rather than memorizing answer templates.

    \item \textbf{Group-Relative Discrimination (Lemma~\ref{lem:gap_expansion}):} GRPO's group-relative normalization naturally amplifies the discriminative power of critiques. By centering around $\bar{r}_G$, the update focuses on \textit{relative} differences. Critiques enhance these differences by providing orthogonal structural information, breaking ties among responses with similar scalar rewards.

    \item \textbf{Bias-Free Integration (Lemma~\ref{lem:bias_free}):} Unlike methods that train separate reward models from language feedback~\citep{azar2023general}, \textsc{Critique-GRPO} directly uses refinements as pseudo-targets. This avoids the compounding errors inherent in multi-stage pipelines, ensuring that the "Eureka moments" identified via structural elimination are stably internalized.
\end{enumerate}

In summary, our theoretical analysis demonstrates that \textsc{Critique-GRPO} achieves provable improvements over pure reward-based learning by:
\begin{itemize}
    \item Guaranteeing weak dominance in regret (never worse, often better)
    \item Achieving exponential sample complexity reduction in structured domains
    \item Maintaining gradient consistency without auxiliary value functions
\end{itemize}
