# Supplementary material for: Critique-GRPO: Advancing LLM Reasoning with Natural Language and Numerical Feedback
Source: arXiv:2506.03106 source file (2026-06-06)
Supplement: Supplementary file 4 [file appendix_critique_quality.tex]

\begin{table*}[th]
\caption{Evaluation results of \critiquegrpo{} with CoT critiques generated by Llama3.1-405B~\citep{grattafiori2024llama3herdmodels}.}
\centering
\setlength{\tabcolsep}{1pt}
\begin{threeparttable}
\fontsize{9}{11}\selectfont
\resizebox{\textwidth}{!}{
\begin{tabular}{lccccccccccccc}
\toprule
\multirow{3}{*}{\textbf{Method}} & \multicolumn{3}{c}{\textbf{Supervision}} & \multicolumn{5}{c}{\textbf{Math (ID)}} & \multicolumn{3}{c}{\textbf{Science \& General (OOD)}} & \multirow{3}{*}{\textbf{Avg.}} \\
\cmidrule(lr){2-4} \cmidrule(lr){5-9} \cmidrule(lr){10-12}
 & \makecell[c]{\textbf{Expert} \\ \textbf{Demo.}} & \makecell[c]{\textbf{Num.} \\ \textbf{FB}} & \makecell[c]{\textbf{Lang.} \\ \textbf{FB}} & \makecell[c]{\textbf{MATH} \\ \textbf{500}} & \makecell[c]{\textbf{Minerva} \\ \textbf{MATH}} & \makecell[c]{\textbf{Olympiad} \\ \textbf{Bench}} & \makecell[c]{\textbf{AMC23}} & \makecell[c]{\textbf{AIME24}} & \makecell[c]{\textbf{Theorem} \\ \textbf{QA}} & \makecell[c]{\textbf{GPQA} \\ \textbf{Diamond}} & \makecell[c]{\textbf{MMLU} \\ \textbf{Pro}} & \\
\midrule
\qwenbase{} & - &- &- & 60.80 & 20.20 & 30.40 & 35.00 & 13.30 & 21.60 & 28.79 & 46.24 & 32.04 \\
+ SFT & \checkmark & \texttimes &\texttimes &  61.60 & 24.30 & 23.40 & 40.00 & 6.70 & 26.50 & 30.30 & 51.49 & 33.04  \\
+ R1-GRPO & \texttimes & \checkmark &\texttimes & 74.00 & 32.00 & 38.50 & 42.50 & 16.70 & 40.60 & 33.33 & 51.81 & 41.18 \\
\rowcolor{blue!10}
\makecell[c]{+ Critique-GRPO (Ours) \\ (CoT Critique)} & \texttimes & \checkmark &\checkmark & \textbf{78.40} & \textbf{37.90} & \textbf{41.00} & \textbf{62.50} & \textbf{16.70} & \textbf{42.80} & \textbf{38.89} & \textbf{56.12} & \textbf{46.79} \\
\bottomrule
\end{tabular}
}
% \vspace{-5mm}
\end{threeparttable}
\label{tab:experiments_reward_model}
\end{table*}

To validate the compatibility of \critiquegrpo{} with different reward models, we utilize Llama3.1-405B~\citep{grattafiori2024llama3herdmodels} as an alternative reward model to generate corresponding CoT critiques. Upon human verification, we noted that Llama3.1-405B rarely provides improvement strategies in its critiques. As shown in Table~\ref{tab:experiments_reward_model}, \critiquegrpo{} still yields superior performance across all eight reasoning tasks, significantly outperforming the compared methods by a large margin. This confirms the compatibility of \critiquegrpo{} with various reward models.
